# Supplementary material for: A Two-Stage, Model-Based Reinforcement Learning Approach for Active Flow Control of Bluff Body Wakes
Source: arXiv:2609.08436 source file (2026-09-08)
Supplement: Supplementary file 1 [file Appendix.tex]

\newpage

\section*{Appendix}

%\input{MaterialControl.tex}
%\input{Hybrid.tex}
\input{ILQR}
